# Supplementary material for: Accurate Parameter Estimation for Risk-aware Autonomous Systems
Source: arXiv:2006.12687 source file (2022-03-16)
Supplement: Supplementary file 2 [file supplementary.tex]

% %%%%%%%% ICML 2021 EXAMPLE LATEX SUBMISSION FILE %%%%%%%%%%%%%%%%%

% \documentclass{article}

% % Recommended, but optional, packages for figures and better typesetting:
% \usepackage{microtype}
% \usepackage{graphicx}
% \usepackage{subfigure}
% \usepackage{booktabs} % for professional tables


% \usepackage{amsmath}
% \usepackage{amssymb}
% \usepackage{amsthm}

% % hyperref makes hyperlinks in the resulting PDF.
% % If your build breaks (sometimes temporarily if a hyperlink spans a page)
% % please comment out the following usepackage line and replace
% % \usepackage{icml2021} with \usepackage[nohyperref]{icml2021} above.
% \usepackage{hyperref}

% \usepackage{xr-hyper}

% \makeatletter
% \newcommand*{\addFileDependency}[1]{% argument=file name and extension
%   \typeout{(#1)}
%   \@addtofilelist{#1}
%   \IfFileExists{#1}{}{\typeout{No file #1.}}
% }
% \makeatother

% \newcommand*{\myexternaldocument}[1]{%
%     \externaldocument{#1}%
%     \addFileDependency{#1.tex}%
%     \addFileDependency{#1.aux}%
% }

% \myexternaldocument{./main}


% % Attempt to make hyperref and algorithmic work together better:
% \newcommand{\theHalgorithm}{\arabic{algorithm}}

% % Use the following line for the initial blind version submitted for review:
% \usepackage{icml2021}

% % If accepted, instead use the following line for the camera-ready submission:
% %\usepackage[accepted]{icml2021}

% % The \icmltitle you define below is probably too long as a header.
% % Therefore, a short form for the running title is supplied here:
% \icmltitlerunning{Appendix}

% \input{utils-supplementary}


% \newcommand{\ww}[1]{\textcolor{red}{#1}}


% \begin{document}

% \onecolumn
% \icmltitle{Feasible Parameter Estimation Bounds for Physical Dynamic Systems\\ Based on the Theory of Spectral Lines: Appendix}
           
           
% % It is OKAY to include author information, even for blind
% % submissions: the style file will automatically remove it for you
% % unless you've provided the [accepted] option to the icml2021
% % package.

% % List of affiliations: The first argument should be a (short)
% % identifier you will use later to specify author affiliations
% % Academic affiliations should list Department, University, City, Region, Country
% % Industry affiliations should list Company, City, Region, Country

% % You can specify symbols, otherwise they are numbered in order.
% % Ideally, you should not use this facility. Affiliations will be numbered
% % in order of appearance and this is the preferred way.
% \icmlsetsymbol{equal}{*}

% \begin{icmlauthorlist}
% \icmlauthor{Arnab Sarker}{mit}
% \icmlauthor{Joseph E. Gaudio}{mit}
% \icmlauthor{Anuradha M. Annaswamy}{mit}
% \end{icmlauthorlist}

% \icmlaffiliation{mit}{Massachusetts Institute of Technology, Cambridge, MA, USA}

% \icmlcorrespondingauthor{Arnab Sarker}{arnabs@mit.edu}

% % You may provide any keywords that you
% % find helpful for describing your paper; these are used to populate
% % the "keywords" metadata in the PDF but will not be shown in the document
% \icmlkeywords{Machine Learning, ICML}

% \vskip 0.3in
% \appendix
% \paragraph{Organization of the appendix.}

% We discuss the continuous time analogue to Section \ref{ss:adaptive_preliminaries} in Appendix \ref{a:continuous-background}, to help inform the reader of well-studied contexts for parameter convergence discussed in the adaptive control literature. Probabilistic inequalities are provided in Appendix \ref{a:prob-inequalities}, which are used in Appendices \ref{a:transfer-proof}, \ref{a:s-to-pe}, and \ref{a:unmodeled-proof} to provide detailed proofs of claims. Appendix \ref{a:experiment-details} discusses specific details and parameter selections with respect to the experiments shown in the paper.

% \section{Time-Varying Regression in Continuous Time}
% \label{a:continuous-background}
% \input{appendix/continuous-background}

% \section{Probabilistic Inequalities}
% \label{a:prob-inequalities}
% \input{appendix/prob-inequalities.tex}

% \section{Proof of Lemma \ref{spectral-transfer}}
% \label{a:transfer-proof}
% \input{appendix/transfer-proof}

% \section{Proof of Proposition \ref{spectral-to-PE}}
% \label{a:s-to-pe}
% \input{appendix/spectral-to-pe-proof.tex}

% % \section{Proof of Theorem \ref{system-id-thm}}
% % \label{a:si-proof}
% % \input{appendix/main-thm-proof.tex}

% \section{Proof of Theorem \ref{unmodeled-estimation}}
% \label{a:unmodeled-proof}
% \input{appendix/unmodeled-proof.tex}

% \section{Experiment Details}
% \label{a:experiment-details}
% \input{appendix/experiment-details.tex}

% \bibliographystyle{icml2021}
% \bibliography{main}

% \end{document}
